# Supplementary material for: Collaborative Learning for Enhanced Unsupervised Domain Adaptation
Source: arXiv:2409.02699 source file (2025-04-16)
Supplement: Supplementary file 1 [file X_suppl.tex]

\clearpage
\setcounter{page}{1}
\maketitlesupplementary

\section{Overview of Supplementary}
This supplementary material presents detailed analyses, algorithm, and qualitative comparison with previous works.  All experiments were conducted using the same hyperparameters and setting as presented in the main paper. \\

\begin{itemize}
    \item Additional aspects of the collaborative learning (Sec.~\ref{sup: analysis}) \\
    \item Additional ablation study (Sec.~\ref{sup: abl}) \\
    \item Overall algorithm of CLDA (Sec.~\ref{sup: algo}) \\
    \item Representation Disparity in layer-wise relation (Sec.~\ref{sup:tsne}) \\
    \item Qulitative comparison with previous works (Sec.~\ref{sup: comparison})
\end{itemize}
% $Z=v\times v$

\section{Analysis for Collaborative Learning} 
\label{sup: analysis}

%=========================================================================

To address the DSN problem, it is crucial to build a computationally efficient layer-wise relations while effectively utilize the layers of the student model that are less affected by the DSN problem. Understanding the information exchange and interaction between the two models is essential for this purpose. With this understanding, the teacher model can effectively incorporate the strengths of the student model while maintaining an acceptable computational cost, thereby deriving the optimal solution to the DSN problem. Key findings from our additional analysis are summarized as follows:
\begin{itemize}
     \item {\bf Teacher to Student}: Knowledge transfer from the teacher to the student (T $\rightarrow$ S) has a significant impact on the attention module, and this effect becomes more pronounced as the layer depth increases.
    \item {\bf Student to Teacher}: When updating the teacher from the student (S $\rightarrow$ T), a channel similarity-based approach proves to be effective.
\end{itemize}

% Fig 1 ===================================================================
\begin{figure}[t!]
\centering
\includegraphics[width=0.7 \columnwidth,height=0.55 \columnwidth]{ICCV2025-Author-Kit/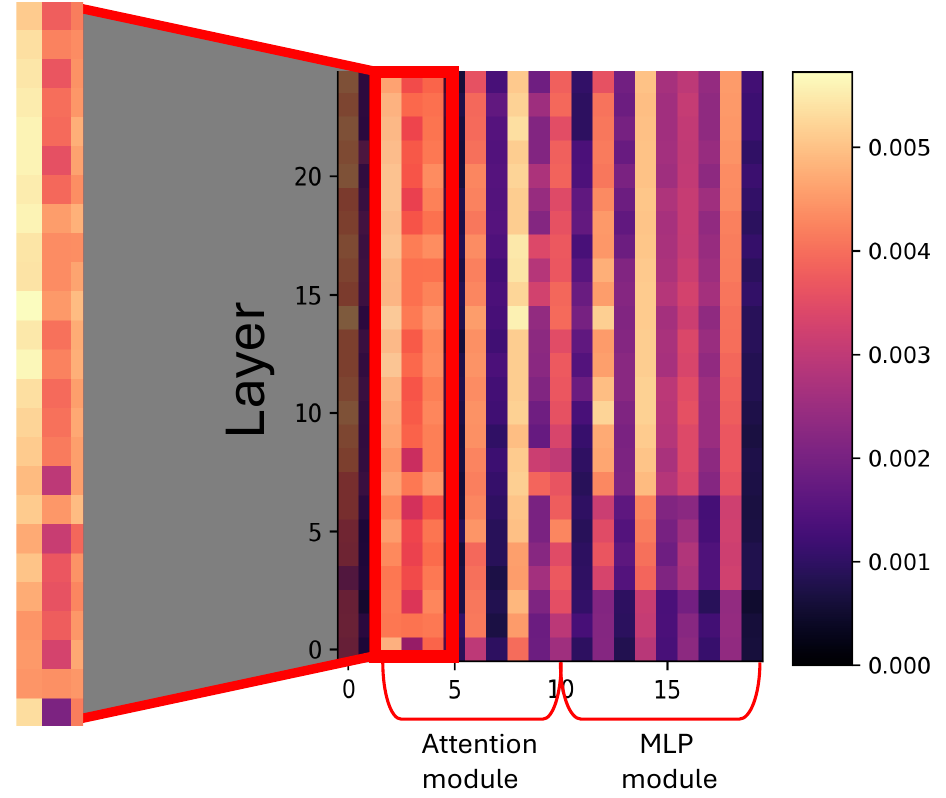} 
\caption{ { \bf PVR heatmap between the distilled student (S) and the independent student(IS). }The heat map shows the average pixel variation rates (PVR) between the distilled student(S) and independent student model(IS), with brighter areas indicating larger value differences. Knowledge transfer from the teacher to the student (T $\rightarrow$ S) has a significant impact on the attention module, and this effect becomes more pronounced as the layer depth increases.}
\label{analysis:fig4}
\end{figure}
%==========================================================================

\subsection{Teacher to Student}
Initially, we investigate the changes when knowledge was transferred from the teacher model to the student model. Our hypothesis posited that when the teacher model exerts greater influence on certain modules of the student model, notable changes in the parameters of those modules are observed compared to a independent student(IS). To validate this, we measured the average per-pixel variation rate (PVR) across modules within the layer, such as attention module and mlp module, between the distilled student model $f_{S}$ and the independently trained student model $f_{IS}$ as follows:\

\begin{equation}
PVR (f,\phi^{(m)} ) = \frac{\sum_{d = 0}^{D}\left| \phi_{IS,d}^{m} - \phi_{S,d}^{m}\right|}{D}\,.
\label{eq:PVR}
\end{equation}

\noindent  where $\phi^{i,m}$ denotes the weight for module $m$ within layer $i$, $D$ represents the dimensions of module $m$.  In Fig.~\ref{analysis:fig4}, we identified two key findings. First, the Attention module was found to be more affected than the MLP module. 
Second, the distilled student exhibited increasingly pronounced effects as the network depth increased. These results suggest a need to design collaborative learning strategies particularly in the attention modules and the deeper layers of the model, where the teacher's knowledge has substantial impact.

\begin{figure}[t!]
\centering
\includegraphics[width=0.75 \columnwidth,height=0.6 \columnwidth]{ICCV2025-Author-Kit/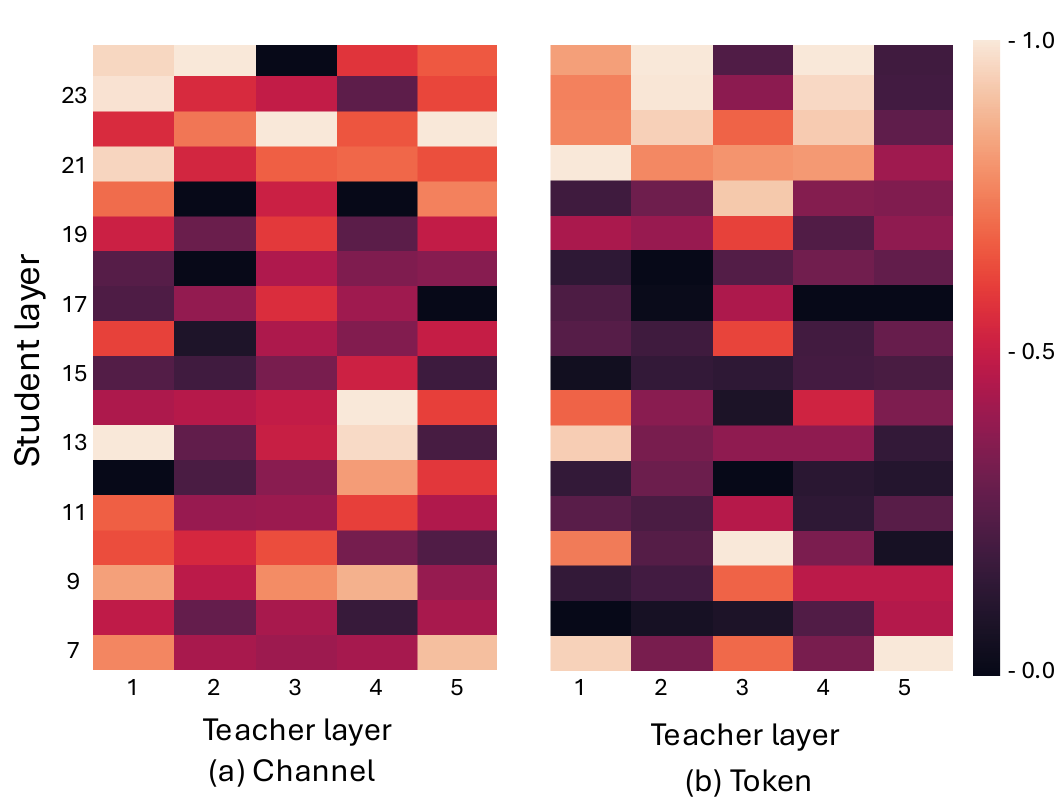} 
\caption{{\bf Comparison of cosine similarity between teacher (T) and distilled student model(S): Channel vs. Token relations.} (a) The heat map presents the cosine similarity measured between the feature maps of the teacher(T) and distilled student models (S), based on channel relations. (b) presents the results of a similar measurement between the two feature maps, but based on token relationships. Instead of measuring similarity across all layers in the student model, we focused on evaluating similarity within the feature maps of the deeper layers (7–24 layers).}
\label{analysis:fig5}
\end{figure}

\subsection{Student to Teacher}
Based on the aforementioned observations, it is a reasonable choice to update the teacher model by leveraging the student model in areas where active interaction occurs. To determine the optimal layer in the student's attention module that corresponds to the teacher model, we carefully considered three key aspects: 1) Token-wise relationships, 2) Channel-wise relationships, and 3) Combining both 1 and 2. We measure each relationship as cosine similarity for the attention feature map in the student's layer based on a randomly selected non-salienct layer of the teacher. As shown in Fig.~\ref{analysis:fig5} (b), examining the token-wise relationships reveals that most layers exhibit low similarity and inconsistent similarity distributions. In contrast, the channel-wise relationships Fig.~\ref{analysis:fig5} (a) show a consistent distribution.
Detailed experimental results can be found in Sec~\ref{sup: abl}.
Based on these findings, the following design principle is derived: during the teacher update (S $\rightarrow$ T), efficient collaborative learning can be achieved by carefully considering channel similarity between the two models within the feature maps of the attention modules in the deeper layers, rather than across all layers.

\section{Additional ablation study} \label{sup: abl}
\paragraph{Layer-wise relation :} In the previous chapter, we analyzed the relation between the student and teacher models from three perspectives: 1) token-wise, 2) channel-wise, and 3) a combination of both. To gain deeper insights, we conducted experiments on the GTA to Cityscapes with DAFormer[MiT-b3], in Tab.~\ref{tab:relation3}. When measuring the similarity of the feature maps between the two models at the token level (Row 1), we observed a performance decrease of 0.5\% compared to the scenario where knowledge was transferred from teacher to student. This decline is attributed to the difficulty of identifying the appropriate student layer for updating, as token-wise approach failed to capture the correct relational context. Conversely, the channel-wise approach (row2) led to the update of suitable layers, resulting in a performance improvement of 1.4\% over the DAFormer. When considering both token-wise and channel-wise relationships, the performance improved compared to the token-wise approach but did not surpass the results achieved with channel-wise approach.
%=====================================================
\begin{table}[t]
%\resizebox{\paperwidth}
\caption{Ablation study on the different layer-relation building.}
\label{tab:relation3}
\centering
\small\addtolength{\tabcolsep}{5pt}
\begin{tabular}{l|c}
\toprule                                        
Method                        & mIoU  \\
\midrule       
token-wise &  68.4 \%  \\
\rowcolor{gray!20} channel-wise &  69.5 \%  \\
both &  68.5 \%  \\ 

\bottomrule
\end{tabular}
\vspace{-0.3cm}
\end{table}
%====================================================

%======================================================
\section{Algorithm}
\label{sup: algo}

\begin{algorithm}[h]
\caption{{\bf C}ollaborative {\bf L}earning for enhanced {\bf D}omain {\bf A}daptation (CLDA)}
\label{alg:clda}
\begin{algorithmic}[1]
\Require 
\begin{itemize}
    \item Teacher network $f_{T}$, Student network $f_{S}$
    \item Early KD training stage $T_0$, layer-wise relation stage $T_{LR}$
    \item Total iterations $T$
    \item Parameters $\phi_S,\theta_S$ of the student model
    \item Parameters $\phi_T,\theta_T$ of the teacher model
\end{itemize}
\Ensure 
\For{$t = 0$ to $T$}
    \State /* \textit{Knowledge Distillation} (T $\rightarrow$ S) */
    \State \textbf{Compute} $L_{CLDA}$ using $\phi_S,\theta_S$ of the student model
    \State \textbf{Update} student parameters $\phi_S,\theta_S$ with $L_{CLDA}$
    \vspace{7pt}
    
    \State /* \textit{Layer-wise relation} */    
    \If{$T_0 \le t  \le T_{LR}$}
        \State \textbf{Identify} non-salient layer $\gamma$ using Eq.~\eqref{eq:LSR}
        \State \textbf{Compute} similarity score $\vartheta$ using Eq.~\eqref{eq:layer_mapping}      
    \EndIf

    \If{$t = T_{LR}$}
        \State \textbf{Compute} student layer $i^{*}$ using Eq.~\eqref{eq:layer_index}
    \EndIf
    \vspace{7pt}
    
    \State /* \textit{Teacher Update} (S $\rightarrow$ T) */
    \If{$t > T_{LR}$}
        \State \textbf{Update} $\phi_{T,\gamma} \leftarrow \alpha \phi_{T,\gamma} + (1 - \alpha)\phi_{S,LS(\gamma)}$
    \EndIf
\EndFor
\end{algorithmic}
\end{algorithm}
%===============================================

In Algorithm \ref{alg:clda}, we summarize our proposed CLDA framework.
The framework consists of a teacher network $f_T$ and a student network $f_S$, where the teacher initially guides the student’s learning, and the student subsequently refines the teacher’s knowledge through collaborative learning. The training process progresses over \( T \) iterations. In the early KD training stage \( T_0 \), the student network learns from the teacher network using \( L_{distill} \), facilitating adaptation to the target domain. Between \( T_0 \) and \( T_{LR} \), layer-wise relations are established between the teacher's non-salient layers and the student's layers. For \( t > T_{LR} \), based on the established layer-wise relations, the teacher's non-salient layers are progressively updated by the student, while simultaneously transferring enhanced knowledge to the student network.
%----------------------------------------------------------

%=========================================================
\begin{figure}[t!]
\begin{center}
\includegraphics[width=1\linewidth]{ICCV2025-Author-Kit/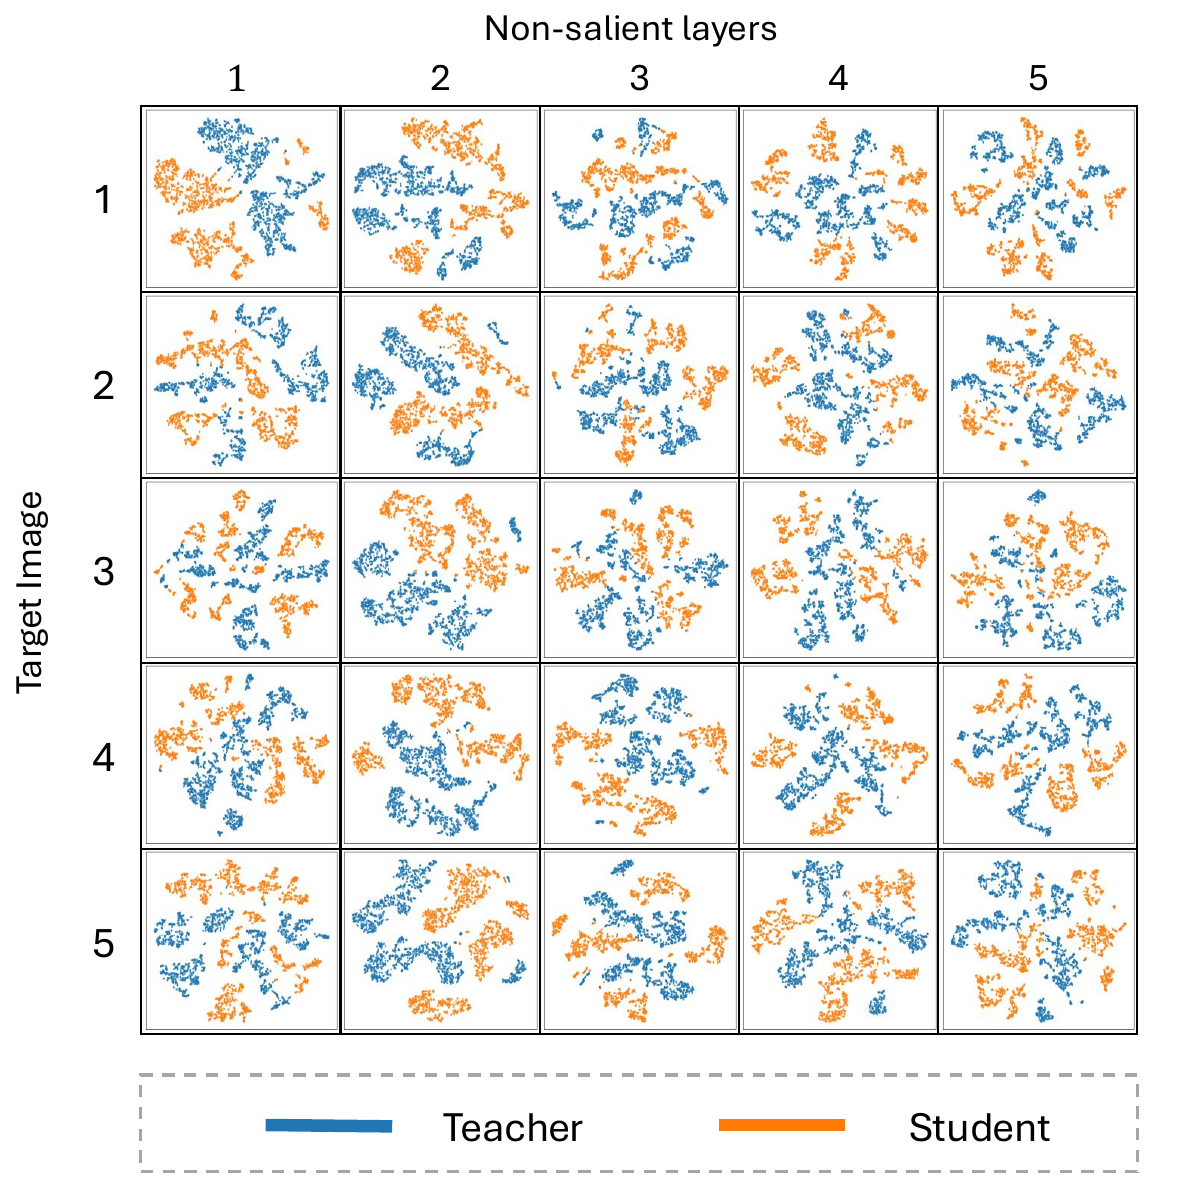}
\end{center}
\vspace{-15pt}
\caption{{\bf T-SNE Visualization of features from the teacher’s non-salient layers and the identical student layer (same size) }: 
Using T-SNE~\cite{van2008visualizing}, we visualized the features of the non-salient layers of the teacher model and the identical layers of the student model~(same size) on the target image.}  
\label{fig:visualize_tsne_b} 
\end{figure}
% visualization ==============================================================
%=========================================================

\section{Representation Disparity in layer-wise relation} \label{sup:tsne}
In the main paper, we demonstrate the validity of updating the teacher's non-salient layers with the most similar layers in the student model. To support this claim, we present feature visualizations using T-SNE~\cite{van2008visualizing}. Fig.~\ref{fig:visualize_tsne_b} and Fig.~\ref{fig:visualize_tsne_c} compare the feature distributions of the teacher’s non-salient layers with different layers in the student model. Specifically, Fig.~\ref{fig:visualize_tsne_b} visualizes the features extracted from the student model’s layers that have the same size as the teacher model’s layers, while Fig.~\ref{fig:visualize_tsne_c} visualizes the features from the compact student layers that most closely resemble the teacher’s non-salient layers. The results show that in Fig.~\ref{fig:visualize_tsne_b}, the teacher and student features form clusters in similar locations. In contrast, in Fig.~\ref{fig:visualize_tsne_c}, the student model’s layer features construct distinct regions separate from the teacher’s non-salient layer features. This suggests that the features between the student layer and the teacher’s non-salient layer (C) exhibit greater variability compared to the features between corresponding layers (B). In other words, even when a student layer shows the highest similarity to a given non-salient teacher layer, it does not merely share the same characteristics but instead exhibits more diverse representation. This allows the student layer to complement the teacher’s non-salient layer by enriching the representation of information that the teacher layer has not sufficiently captured in the target domain. These findings further reinforce the core argument of this paper, providing additional evidence that updating the teacher’s non-salient layer with the most similar layer in the student model is an effective strategy.

%==========================================================================
\begin{figure}[t!]
\begin{center}
\includegraphics[width=1\linewidth]{ICCV2025-Author-Kit/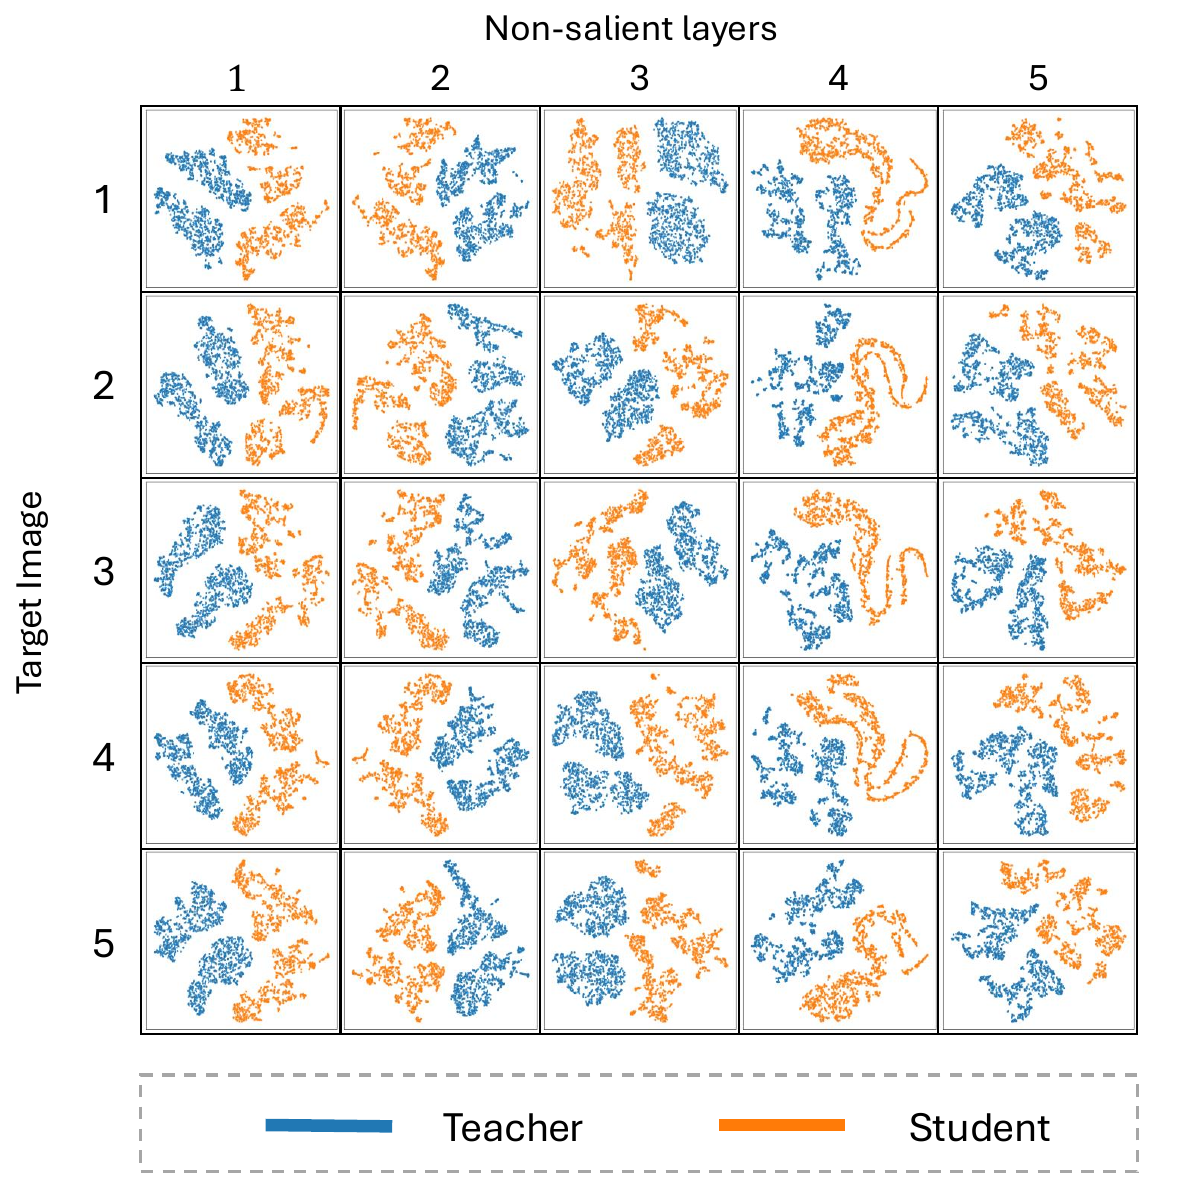}
\end{center}
\vspace{-15pt}
\caption{{\bf T-SNE Visualization of features from the teacher’s non-salient layers and the most similar student layer}: 
The visualization of features from the teacher's non-salient layer and the most similar layer in the student model using T-SNE~\cite{van2008visualizing}. The results show that the most similar student layer does not merely share the same characteristics as the teacher's non-salient layer but instead exhibits greater representational diversity.}  
\label{fig:visualize_tsne_c} 
\end{figure}
% visualization ==============================================================

\begin{figure*}[t!]
\begin{center}
\includegraphics[width=1\linewidth]{ICCV2025-Author-Kit/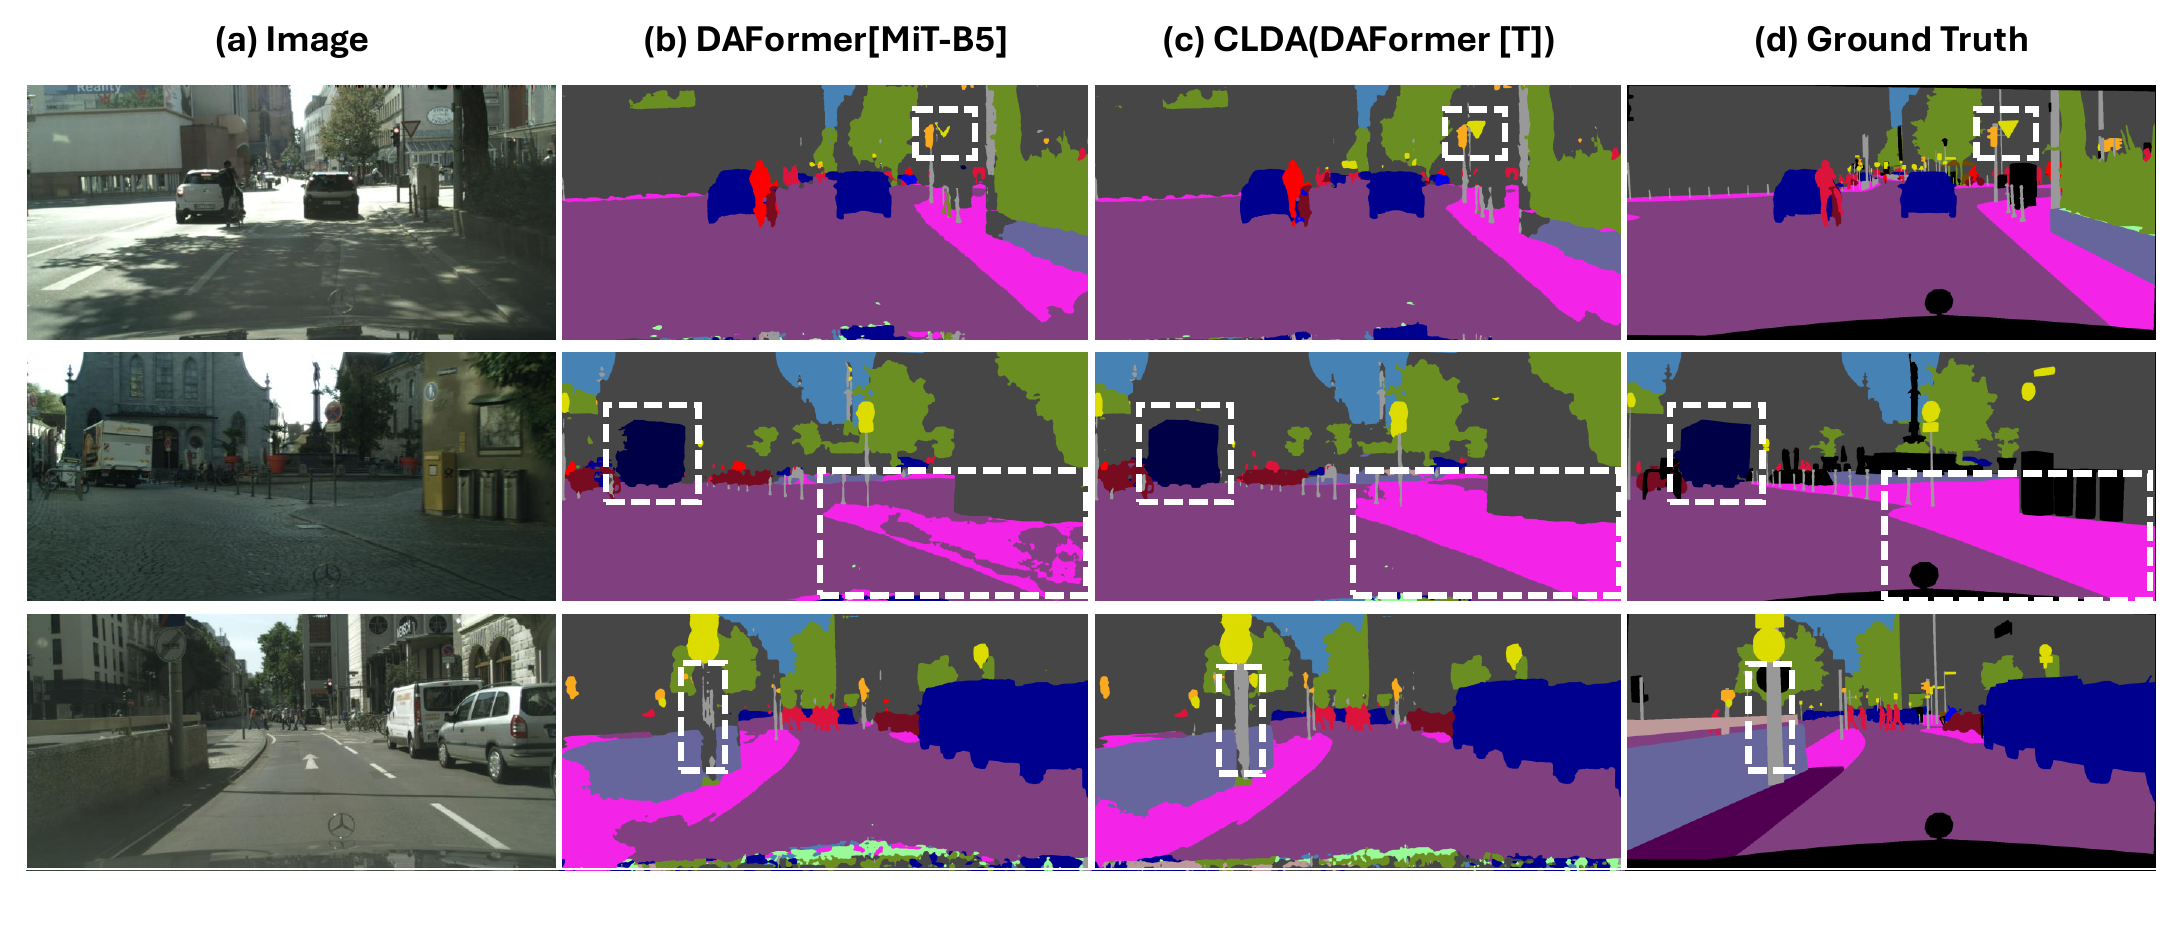}
\end{center}
\vspace{-15pt}
\caption{{\bf Qualitative comparison of CLDA~[T] with DAFormer~[MiT-B5] on GTA→Cityscapes}: (a) target RGB image, (b) our UDA baseline method, DAFormer~[MiT-B5], (c) CLDA~[T], and (d) semantic label.}  
\label{fig:visualize_teacher} 
\end{figure*}

\begin{figure*}[t!]
\begin{center}
\includegraphics[width=1\linewidth]{ICCV2025-Author-Kit/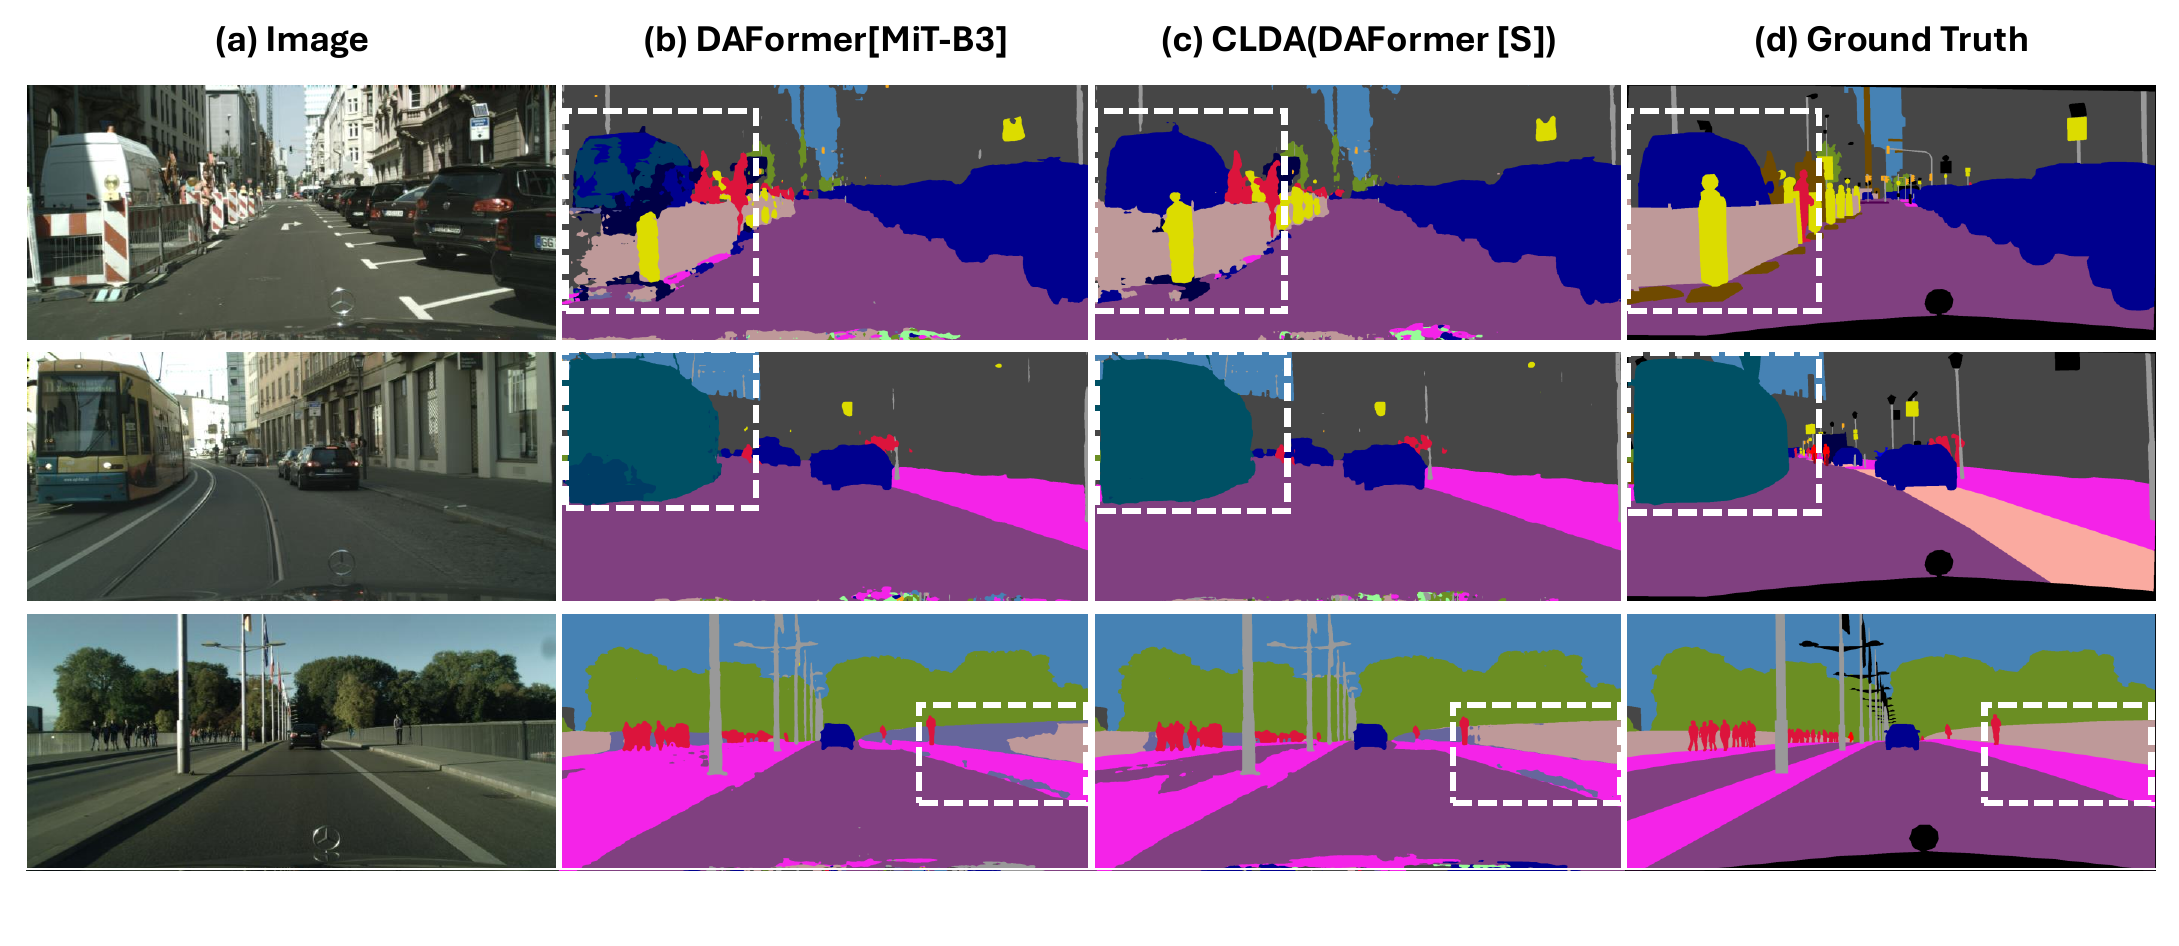}
\end{center}
\vspace{-15pt}
\caption{{\bf Qualitative comparison of CLDA~[S] with DAFormer~[MiT-B3] on GTA→Cityscapes}: (a) target RGB image, (b) our UDA baseline method, DAFormer~[MiT-B3], (c) CLDA~[S], and (d) semantic label.}  
\label{fig:visualize_student} 
\end{figure*}

%=====================================================

\section{Further Example Predictions}
\label{sup: comparison}
To demonstrate the effectiveness of CLDA, we provide additional representative examples in comparison with DAFormer. In the GTA$\rightarrow$Cityscapes semantic segmentation task, both the teacher and student models exhibit significant performance improvements in the fence, pole, traffic sign, truck, and bus classes, as also shown in Tables 1-2 of the main paper. The predictions of the teacher model, presented in Fig.~\ref{fig:visualize_teacher}, illustrate notable improvements in the traffic sign, truck, and pole classes compared to previous methods. In the existing method, there was a problem where traffic signs were mixed with the surrounding background and poles were not properly detected. However, with CLDA, these objects are segmented more clearly. Additionally, for the truck class, the previous method frequently misclassified trucks as cars or confused them with background elements, whereas CLDA successfully distinguishes them, demonstrating a more refined segmentation.
The student model’s predictions, shown in Fig.~\ref{fig:visualize_student}, highlight even greater performance gains in the truck, bus, and fence classes. The previous method struggled to differentiate between trucks and buses and failed to segment fences accurately. However, with CLDA[S], the student model benefits from the enhanced knowledge transferred from the updated teacher model, enabling it to make more accurate predictions. This demonstrates a complementary effect, with the improved performance of the teacher model further enhancing the student model's ability to distinguish classes.
%=====================================================
